# Supplementary material for: Coffee: Boost Your Code LLMs by Fixing Bugs with Feedback
Source: arXiv:2311.07215 source file (2024-02-23)
Supplement: Supplementary file 1 [file gpt4_identification.tex]

\begin{table*}[t]
    \centering
    \small
    \begin{tabular}{p{14cm}}
        \toprule
        \textbf{Prompt} \\
        \midrule
        You will be provided with a description of a problem, wrong code, and the correct code that is intended to solve the issue.\\
        \\
        Along with these, you will receive a feedback addressing the inaccuracies or issues in the wrong code.\\
        \\
        Your task is to carefully evaluate feedback.\\
        \\
        Evaluation Criteria:\\
        \\
        Identification Score (1-5): Assess the accuracy with which the feedback pinpoints the error in the code. Consider the precision of the error identification, ensuring that it is direct and unambiguous.\\
        \\
        The scoring should reflect how well the feedback isolates the mistake and provides a clear understanding of the issue within the code. The scale consists of:\\
        \\
        1. Inadequate Identification: The feedback is off-target, either highlighting a code section that is not at fault or completely overlooking the actual error. This leads to misunderstanding and provides no help in correcting the code.\\
        \\
        2. Rough Identification: The feedback points to a general area that contains the error but is not precise enough, possibly causing confusion by implicating multiple aspects of the code. Additionally, it might acknowledge a less critical issue while omitting the main error.\\
        \\
        3. General Identification: The feedback identifies the correct error but does not pinpoint it with full precision. The feedback is on the right track but lacks the necessary clarity to be completely effective. \\
        \\
        4. Specific Identification: The feedback directly identifies the particular error in the code and explains it with decent clarity. It may be missing an in-depth explanation or guidance for resolution, but the error is correctly and specifically highlighted.\\
        \\
        5. Precise Identification: The feedback accurately isolates the error, providing a detailed and clear indication of the specific issue within the code, enabling efficient correction without ambiguity.\\
        \\
        please evaluate given feedback on evaluation criteria and assign an appropriate score after the SCORE token at the end.\\
        \\
        \textbf{Problem Description:}\\
        \{problem\}\\
        \\
        \textbf{Incorrect Code:} \\
        \{incorrect\_code\} \\
        \\
        \textbf{Correct Code:}\\
        \{correct\_code\}\\
        \\
        \textbf{Feedback:}\\
        \{Feedback\}\\
        \\
        \textbf{SCORE:}\\
        \bottomrule
    \end{tabular}
    
    \caption{\textbf{The Prompt for GPT-4 Evaluation.} We prompt GPT-4 to evaluate the feedback quality on coding errors, focusing on error identification.}
    \label{tab:gpt4_identification}
\end{table*}
