# Supplementary material for: Coffee: Boost Your Code LLMs by Fixing Bugs with Feedback
Source: arXiv:2311.07215 source file (2024-02-23)
Supplement: Supplementary file 2 [file gpt4_guidance.tex]

\begin{table*}[t]
    \centering
    \small
    \begin{tabular}{p{14cm}}
        \toprule
        \textbf{Prompt} \\
        \midrule
        You will be provided with a description of a problem, wrong code, and the correct code that is intended to solve the issue.\\
        \\
        Along with these, you will receive a feedback addressing the inaccuracies or issues in the wrong code.\\
        \\
        Your task is to carefully evaluate feedback.\\
        \\
        Evaluation Criteria:\\
        \\
        Guidance Score (1-5): Does the feedback accurately provide a solution for the error in the code?\\
        \\
        1. Confusing: The feedback does not address the error or provides inaccurate guidance, leading to further confusion or incorrect implementation.\\
        \\
        2. Partially Clear: The feedback partially addresses the error but lacks clarity or specificity, making it challenging to understand or implement the solution correctly.\\
        \\
        3. Adequate: The feedback identifies the error and provides a solution but lacks detail or explanation, requiring additional effort for implementation.\\
        \\
        4. Clear: The feedback accurately pinpoints the error and offers a clear solution with some explanations, aiding in understanding and implementation.\\
        \\
        5. Comprehensive: The feedback precisely identifies the error, provides a comprehensive solution with clear explanations and examples, making it easy to understand and implement the fix.\\
        \\
        Provide a detailed assessment of feedback given evaluation criteria and assign an appropriate score after the SCORE token at the end.\\
        \\
        \textbf{Problem Description:}\\
        \{problem\}\\
        \\
        \textbf{Incorrect Code:} \\
        \{incorrect\_code\} \\
        \\
        \textbf{Correct Code:}\\
        \{correct\_code\}\\
        \\
        \textbf{Feedback:}\\
        \{Feedback\}\\
        \\
        \textbf{SCORE:}\\
        \bottomrule
    \end{tabular}
    
    \caption{\textbf{The Prompt for GPT-4 Evaluation.} We prompt GPT-4 to evaluate the feedback quality on coding errors, focusing on providing guidance given errors.}
    \label{tab:gpt4_guidance}
\end{table*}
